# Supplementary material for: Vulnerability of fault-tolerant topological quantum error correction to quantum deviations in code space
Source: arXiv:2301.12859 source file (2025-03-08)
Supplement: Supplementary file 1 [file SuppInfo-LGT.pdf]

# Supplemental Information for "Lattice Gauge Theory and Topological Quantum Error Correction with Quantum Diversions in the Error Detection"

In this supplemental information, we provide details about derivations of the results in the main text. In Sec. [SI](#) we discuss some properties about code space when initial state preparation suffers from imperfection measurement. In Sec. [SII](#) we derive the SM mapping explicitly. In Sec. [SIII](#) we talk about the consequence of local symmetry under the Nishmori condition. In sec. [SIV](#) we derive the low-temperature expansion of the Wilson loop.

## SI. CODE SUBSPACE UNDER IMPERFECT MEASUREMENT

Here we discuss the imperfect code subspace under the presence of coherent errors on entanglement gates during state preparation. Starting with a product state  $\bigotimes_{e_0} |+\rangle_{e_0}$ , we obtain the (unnormalized) state  $M_{\{s_{p_0}\}} \bigotimes_{e_0} |+\rangle_{e_0}$  with probability

$$P(\{s_{p_0}\}) = \bigotimes_{e_0} \langle +|_{e_0} E_{\{s_{p_0}\}} \bigotimes_{e_0} |+\rangle_{e_0} = \frac{1}{(8 \cosh \beta)^N} \mathcal{Z}_{\{s_{p_0}\}}, \quad (\text{S1})$$

$$\mathcal{Z}_{\{s_{p_0}\}} = \sum_{\{\sigma_{e_0}\}} \exp \left[ \beta \sum_{p_0} s_{p_0} b_{p_0} \right], b_{p_0} = \prod_{e_0 \in \partial p_0} \sigma_{e_0}, \quad (\text{S2})$$

where  $M_{\{s_{p_0}\}}$  is the imperfect measurement operator

$$M_{\{s_{p_0}\}} = \frac{1}{(\sqrt{2} \cosh \beta)^N} \exp \left[ \frac{1}{2} \beta \sum_{p_0} s_{p_0} B_{p_0} \right], \quad (\text{S3})$$

and  $E_{\{s_{p_0}\}} = M_{\{s_{p_0}\}}^\dagger M_{\{s_{p_0}\}}$  is the corresponding POVM operator. By expanding  $\bigotimes_{e_0} |+\rangle_{e_0}$  under computational basis  $\bigotimes_{e_0} |+\rangle_{e_0} = (1/2^N) \sum_{\{\sigma_{e_0}\}} \bigotimes_{e_0} |\sigma_{e_0}\rangle$ , where  $\sigma_{e_0} = \pm 1$  is the eigenvalue of Pauli operator  $Z_{e_0}$ , it can be shown that  $P(\{s_{p_0}\})$  is proportional to the partition function of a 2-d  $\mathbb{Z}_2$  lattice gauge theory  $\mathcal{Z}_{\{s_{p_0}\}}$  [\[1, 2\]](#), which is a useful method to dealing with the post-measurement state and is helpful to our following derivations. Note that 2-d  $\mathbb{Z}_2$  lattice gauge theory is exact-solvable [\[3\]](#). By noticing that the Boltzmann weight only depends on the value of  $b_{p_0}$ , we rewrite the summation of spin configurations as a summation of  $b_{p_0}$  configurations together with 1-form symmetry operations

$$\sum_{\{\sigma_{e_0}\}} = \sum_{\{b_{p_0}\}} \delta_{\prod_{p_0} b_{p_0}, 1} \sum_{\text{dual loop}}. \quad (\text{S4})$$

Here  $\delta_{\prod_{p_0} b_{p_0}, 1}$  means that the product of all  $b_{p_0}$  must equal to 1, since the lattice is embedded in a torus surface. We may check the degree of freedoms involved in the summation  $2^{2N} = 2^N/2 \times 2^{N+1}$ . Thus we have

$$\begin{aligned} \mathcal{Z}_{\{s_{p_0}\}} &= \sum_{\{b_{p_0}\}} \delta_{\prod_{p_0} b_{p_0}, 1} \sum_{\text{dual loop}} \exp \left[ \beta \sum_{p_0} s_{p_0} b_{p_0} \right] \\ &= 2^{N+1} \sum_{\{b_{p_0}\}} \frac{1 + \prod_{p_0} b_{p_0}}{2} \exp \left[ \beta \sum_{p_0} s_{p_0} b_{p_0} \right] \\ &= 2^N \prod_p \left( \sum_{b_{p_0}} \exp [\beta s_{p_0} b_{p_0}] + \sum_{b_{p_0}} b_{p_0} \exp [\beta s_{p_0} b_{p_0}] \right) \\ &= 2^N (2 \cosh \beta)^N + 2^N (2 \sinh \beta)^N \prod_{p_0} s_{p_0}, \end{aligned} \quad (\text{S5})$$

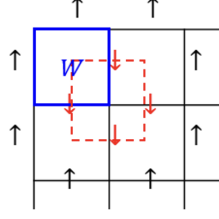

FIG. S1. 2-d  $\mathbb{Z}_2$  lattice gauge theory. The classical spins  $\sigma_{e_0}$  are associated with each edge. Both the Hamiltonian and Wilson loop (blue solid loop) are invariant under 1-form symmetry operation (red dashed loop) which flips the spins on a dual loop.

and hence we have the probability of measurement outcomes

$$P(\{s_{p_0}\}) = \frac{1 + (\tanh \beta)^N \prod_p s_{p_0}}{2^N}. \quad (\text{S6})$$

Note that  $\prod_{p_0} s_{p_0}$  is the parity of  $\{s_{p_0}\}$  configuration.

From the above discussion, it can be seen that we might get different states with respect to the ancilla measurement outcome  $\{s_{p_0}\}$ . But we will fix the initial state as  $M_{\{+\}} \otimes_{e_0} |+\rangle_{e_0}$ , where we assumed the measurement outcomes of ancilla qubits are all +1. For other measurement outcomes  $\{s_{p_0}\}$ , we can redefine the sign of our stabilizers  $B_{p_0} \rightarrow s_{p_0} B_{p_0}$  in order that the following discussions still apply. The only thing we should take into consideration is the parity of outcome  $\{s_{p_0}\}$  because under the redefinition  $\prod_{p_0} B_{p_0} = 1 \rightarrow \prod_{p_0} B_{p_0} = \prod_s s_{p_0}$  and we will get  $-1$  for odd parity. In the odd parity case, the defects on the lattice cannot be paired up and it is unfriendly to error correction. Hence we ignore odd parity outcomes. We might consider it as a post-selection procedure, which chooses the even parity result that occurs with probability  $P_+ = (1 + (\tanh \beta)^N)/2$ , see Eq. (S6). We find that  $1/2 \leq P_+ \leq 1$  for  $0 \leq \beta \leq +\infty$ . Note that this probability is close to 1 we  $\beta$  is sufficiently large, so the post-selection procedure is reasonable for experimental consideration.

Till now we have only obtained one logical state. What about other states in the imperfect code subspace? The problem is that the matrix rank of  $M_{\{s_{p_0}\}}$  is  $2^{2N}$ , which means that if we view it as a map defined on the whole  $2^{2N}$  dimensional Hilbert space of physical qubits,  $M_{\{s_{p_0}\}} : \mathcal{H} \rightarrow \mathcal{H}$ , then we find that  $\text{Im}(M_{\{s_{p_0}\}}) = \mathcal{H}$ . This is different from the projective measurement case that  $P_{\{s_{p_0}\}} = \prod_{p_0} (I + s_{p_0} B_{p_0})/2$  projects any states into the  $B_{p_0} = s_{p_0}$  subspace. That is why we define the code space using logical operators in analogy to experimental setups. In summary, our four logical basis states are defined as

$$\begin{aligned} |\widetilde{++}\rangle &= \frac{M_{\{+\}} \otimes_{e_0} |+\rangle_{e_0}}{\sqrt{\otimes_{e_0} \langle +|_{e_0} M_{\{+\}}^\dagger M_{\{+\}} \otimes_{e_0} |+\rangle_{e_0}}}, \\ |\widetilde{-+}\rangle &= Z_{l_1} |\widetilde{++}\rangle, \quad |\widetilde{+-}\rangle = Z_{l_2} |\widetilde{++}\rangle, \quad |\widetilde{--}\rangle = Z_{l_1} Z_{l_2} |\widetilde{++}\rangle, \end{aligned} \quad (\text{S7})$$

Notice that  $|\widetilde{++}\rangle$  state correspond to the model

$$\mathcal{Z}_{\{+\}} = \sum_{\{\sigma_{e_0}\}} \exp \left[ \beta \sum_{p_0} b_{p_0} \right]. \quad (\text{S8})$$

Given the above imperfect logical states, the expectation value of Pauli  $Z$  operators can be computed through the classical SM model [1, 2]. We denote  $\langle \cdot \rangle_{\{+\}}^q$  as the expectation value of the post-measurement state  $|\widetilde{++}\rangle$ , then

$$\left\langle \prod_{e_0 \in c_0} Z_{e_0} \right\rangle_{\{+\}}^q = \left\langle \prod_{e_0 \in c_0} \sigma_{e_0} \right\rangle_{\{+\}}^c. \quad (\text{S9})$$

where we denote  $c_0$  as a set of several edges and  $\langle \cdot \rangle_{\{+\}}^c$  as the expectation value of the classical model  $\mathcal{Z}_{\{+\}}$ .

2-d  $\mathbb{Z}_2$  lattice gauge theory possesses 1-form symmetry [3]. As in Fig. S1, if we flip all the spins along a dual loop, it does not change the value of  $b_{p_0}$  on any plaquette  $p_0$ , hence does not change the partition function, i.e. Eq. (S2).

For 2-d  $\mathbb{Z}_2$  lattice gauge theory, Elitzur's theorem [3, 4] states that the expectation value of any observable that

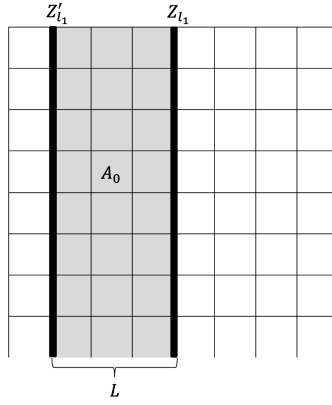

FIG. S2. Different definitions of logical Pauli  $Z$  operator. Under imperfect measurement preparation, the two logical states defined by them are different. The fidelity between these two states relates to the expectation value of a Wilson loop observable constituted by these two non-contractible loops.

varies under 1-form symmetry operation vanishes (even under the presence of infinitesimal source term). For example, consider the overlap between two logical states

$$\langle \widetilde{-+} | \widetilde{++} \rangle = \langle \widetilde{++} | Z_{l_1} | \widetilde{++} \rangle = \langle Z_{l_1} \rangle_{\{+\}}^q = \left\langle \prod_{e_0 \in l_1} \sigma_{e_0} \right\rangle_{\{+\}}^c. \quad (\text{S10})$$

The operator  $\prod_{e_0 \in l_1} \sigma_{e_0}$  is the product  $\sigma_{e_0}$  spins that win around the non-contractible loop  $l_1$ , and it changes sign under the 1-form symmetry operation that flips the spins on a dual non-contractible loop  $l_1^*$  that intersect with  $l_1$ . Consequently, we find that  $\langle \widetilde{-+} | \widetilde{++} \rangle = 0$ . Note that this result can also be checked through explicit calculation since  $Z_{\{+\}}$  acquires an exact solution. Similarly, we find that all the four states  $\{|\widetilde{++}\rangle, |\widetilde{-+}\rangle, |\widetilde{+-}\rangle, |\widetilde{--}\rangle\}$  are orthogonal to each other. Therefore, they form an orthonormal basis of a 4 dimensional subspace. This justifies our definition of the imperfect code subspace

$$\tilde{\mathcal{C}}(\beta) = \text{span}\{|\widetilde{++}\rangle, |\widetilde{-+}\rangle, |\widetilde{+-}\rangle, |\widetilde{--}\rangle\} \quad (\text{S11})$$

What is more, these four states are still eigenstates of logical  $X$  operators. Since  $X_{l_1^*}, X_{l_2^*}$  commute with imperfect measurement operator  $M_{\{+\}}$  and act as 1 on the initial product state, we find that  $X_{l_1^*} |\widetilde{++}\rangle = |\widetilde{++}\rangle, X_{l_2^*} |\widetilde{++}\rangle = |\widetilde{++}\rangle$ . The act on the other three states is determined by the commutation relation between logical  $X$  and logical  $Z$ . Note that these properties are not universal for imperfect measurement but depend on the specific measurement protocol.

Here we point out that, unlike the projective measurement case,  $\tilde{\mathcal{C}}$  depends on the choice of logical operators on the lattice. For example, consider a different choice of logical  $Z$  operator  $Z'_{l_1}$  as in Fig. S2. We can calculate the fidelity between  $|\widetilde{-+}\rangle$  and the new state defined by the new logical operator  $|\widetilde{-+}\rangle' = Z'_{l_1} |\widetilde{++}\rangle$ :

$$\langle \widetilde{-+} | \widetilde{-+} \rangle' = \langle \widetilde{++} | Z_{l_1} Z'_{l_1} | \widetilde{++} \rangle = \langle Z_{l_1} Z'_{l_1} \rangle_{\{+\}}^q \quad (\text{S12})$$

Note that  $Z_{l_1} Z'_{l_1}$  forms a Wilson loop that could be written as the boundary of a region  $A$ . For the classical model, Wilson loops are 1-form symmetry invariant observables and acquire non-zero expectation values. For example, consider the Wilson loop

$$W_{A_0} = \prod_{p_0 \in A_0} b_{p_0} = \prod_{e_0 \in \partial A_0} \sigma_{e_0}, \quad (\text{S13})$$

where  $A_0$  is a 2-d region (a set of plaquettes) and  $\partial A_0$  is the set of edges at the boundary of  $A_0$ . Its expectation value can be evaluated similarly as the partition function, which leads to

$$\langle W_{A_0} \rangle_{\{+\}}^c = \frac{(\tanh \beta)^{|A_0|} + (\tanh \beta)^{N-|A_0|}}{1 + (\tanh \beta)^N}. \quad (\text{S14})$$

With the help of Eq. (S14), we obtain:

$$\langle \widetilde{-+} | \widetilde{-+} \rangle' = \frac{(\tanh \beta)^{dL} + (\tanh \beta)^{N-dL}}{1 + (\tanh \beta)^N} \quad (\text{S15})$$

which is smaller than 1 for finite  $\beta$ , implies that the two states are different.

In addition, notice that we can take the product of the eigenstates of  $N-1$   $B_{p_0}$  operators,  $N-1$   $A_{v_0}$  operators, and 2 logical operators  $X_{l_1^*}$  and  $X_{l_2^*}$  to form a complete basis of the whole Hilbert space of physical qubits. Under this basis the product  $|+\rangle$  state can be written as

$$\bigotimes_{e_0} |+\rangle_{e_0} = \bigotimes_{p_0}' \sum_{b_{p_0}=\pm} |B_{p_0}=b_{p_0}\rangle \bigotimes_{v_0}' |A_{v_0}=+\rangle \bigotimes |X_{l_1^*}=+\rangle \bigotimes |X_{l_2^*}=+\rangle, \quad (\text{S16})$$

Here the prime on the product symbol means that a chosen plaquette or vertex is excluded to satisfy the global constrain  $\prod_{p_0} B_{p_0} = \prod_{v_0} A_{v_0} = I$ . This formula is verified as follows. Since the action of  $A_{v_0}$ 's and logical  $X$  operators on  $\bigotimes_{e_0} |+\rangle_{e_0}$  all yield +1, the state must be the +1 eigenstate of these operators. Besides, assume the excluded plaquette is  $f_0$ . Consider a Pauli  $X$  string  $X_{(f_0 \rightarrow q_0)}$  that starts at  $f_0$  and ends at some other plaquette  $q_0$ . Since  $X_{(f_0 \rightarrow q_0)}$  commutes with all  $N-1$   $A_{v_0}$  operators, logical  $X$  operators and  $N-2$   $B_{p_0}$ 's with  $p_0 \neq q_0, f_0$ , it only acts on the factor  $|B_{q_0}=\pm\rangle$  under the above basis. Note that  $X_{(f_0 \rightarrow q_0)}$  anti-commutes with  $B_{q_0}$ , so  $X_{(f_0 \rightarrow q_0)} |B_{q_0}=\pm\rangle = |B_{q_0}=\mp\rangle$ . Since  $X_{(f_0 \rightarrow q_0)} \bigotimes_{e_0} |+\rangle_{e_0} = \bigotimes_{e_0} |+\rangle_{e_0}$ , the product state must be stabilized by  $X_{(f_0 \rightarrow q_0)}$ . Applying such  $X$  strings to all the plaquettes, we find that  $\bigotimes_{e_0} |+\rangle_{e_0}$  is the +1 eigenstate of  $X_{(f_0 \rightarrow q_0)}$  for all  $q_0 \neq f_0$ , which leads to Eq. (S16). With the above considerations, we find that the imperfect measurement operator  $M_{\{s_{p_0}\}}$  only acts on the stabilizer bits ( $|B_{p_0}=\pm\rangle$  and  $|A_{v_0}=\pm\rangle$ ) and logical operators only act on the logical bits ( $|X_{l_1^*}=\pm\rangle$  and  $|X_{l_2^*}=\pm\rangle$ ). Consequently, any state  $|\tilde{\Psi}\rangle$  in the code space  $\tilde{\mathcal{C}}$  can be expanded under the stabilizer basis to achieve the form:

$$|\tilde{\Psi}\rangle \propto \left[ \exp\left(\frac{\beta}{2} \prod_{p_0}' B_{p_0}\right) \bigotimes_{p_0}' \sum_{b_{p_0}=\pm} \exp\left(\frac{\beta}{2} b_{p_0}\right) |B_{p_0}=b_{p_0}\rangle \right] \left[ \bigotimes_{v_0}' |A_{v_0}=+\rangle \right] \bigotimes |L\rangle, \quad (\text{S17})$$

where  $|L\rangle$  represents the logical qubits and is exactly where the logical information is stored.

### SIII. DERIVATION OF STATISTICAL MECHANICAL MAPPING

Recall that we have considered a multi-round error correction protocol [5] under imperfect syndrome measurement, listed as follows:

1. start with an arbitrary state  $|\tilde{\Psi}\rangle$  in  $\tilde{\mathcal{C}}(\beta_0)$ .
2. Probabilistic Pauli  $X$  error acts at each integer valued time  $t = 1, 2, \dots, T$ . The  $X$  error at each physical qubit on each time slice occurs independently with probability  $q$ . Denote the error chain at time  $t$  as  $c_0^*(t)$ .  $c_0^*(t)$  is a set of edges, where the star reminds us that it will be viewed as strings on the dual lattice. The associated Pauli operator is  $X_{c_0^*(t)} = \prod_{e_0 \in c_0^*(t)} X_{e_0}$ .
3. Perform a round of syndrome measurement between each time interval  $[t, t+1]$ . The syndrome measurements are also imperfect and their strength of measurement is set as  $\beta$ . Suppose the measurement outcome at time interval  $[t, t+1]$  is  $\{s_{p_0}(t)\}$ , then the associated action of imperfect measurement is  $M_{\{s_{p_0}(t)\}}$ .
4. After  $T$  rounds of syndrome measurements, we decode and apply Pauli  $X$  correction to the final state. Denote the correction chain as  $c_{0R}^*$  and corresponding correction operator as  $X_{c_{0R}^*}$ .

Notice that with our definition of code space  $\tilde{\mathcal{C}}$ , the imperfection of syndrome measurement only affects syndrome bits but does not disturb logical information. We have known that any state in  $\tilde{\mathcal{C}}$  takes the form as shown in Eq. (S17). Acting successive imperfect measurement operators on it still only affects the stabilizer bits. The logical information  $|L\rangle$  will be left unchanged.

We might represent our error correction procedure as a diagram in Fig. 3(a). We will show that when the error chains at all times and the correction chain together constitute a contractible loop (correction operator and Pauli error

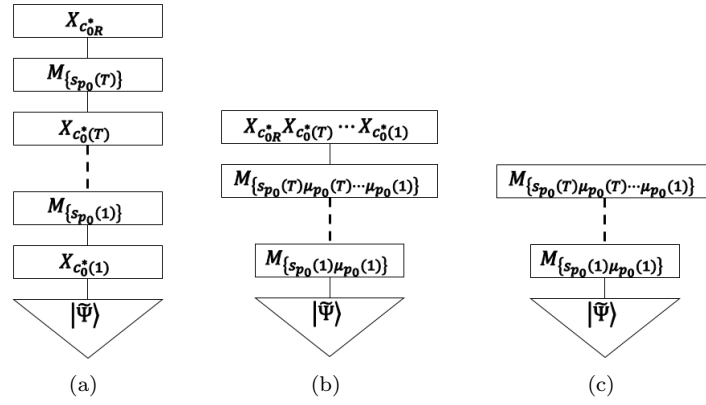

FIG. S3. Diagrams for error correction procedure. The bottom triangle is the initial state. The squares above represent actions of Pauli errors and imperfect measurements. (a) Original error correction procedure. Pauli errors and imperfect measurements act repetitiously. (b) Move Pauli error operators to the top making use of the commutation relation, i.e. Eq. (S18). (c) When the correction operator and Pauli error operators form a stabilizer, they together commute with imperfect measurement operators and hence have no effect on the final state.

operators forms stabilize) the logical information is still preserved. Notice that the commutation between  $M_{\{s_{p_0}(t)\}}$  and Pauli error  $X_{c_0^*}^*(t')$  can be expressed as

$$M_{\{s_{p_0}(t)\}} X_{c_0^*}^*(t') = X_{c_0^*}^*(t') M_{\{s_{p_0}(t)\mu_{p_0}(t')\}}. \quad (\text{S18})$$

Here  $\{\mu_{p_0}(t')\}$  represents the correct syndrome that should be generated by Pauli error  $X_{c_0^*}^*(t')$ . In other words  $\mu_{p_0}(t') = -1$  when  $p$  locates at the boundary of  $c_0^*$  and  $\mu_{p_0}(t') = 1$  otherwise. Using this commutation relation we can move all Pauli error chains in Fig. 3(a) to the top and arrive at Fig. 3(b). When the operator  $X_{c_0^*}^* X_{c_0^*}^*(T) \dots X_{c_0^*}^*(1)$  forms a product of  $A_{v_0}$  operators, it will be commuting with imperfect measurement operators and logical Pauli operators, and hence acts trivially on the state below. Therefore we will obtain a final state as in Fig. 3(c). Though the final state is different from the original state  $|\tilde{\Psi}\rangle$ , it will be containing the same logical information, so we view this situation as a success of error correction.

Then we may compute the probability of syndrome outcomes given a particular error configuration  $\{c_0^*(t)\}$

$$\begin{aligned} P(\{s_{p_0}(t)\}|\{c_0^*(t)\}) &= \|\prod_t M_{\{s_{p_0}(t)\}} X_{c_0^*}^*(t) |\tilde{\Psi}\rangle\|^2 \\ &= \|\prod_t M_{\{s_{p_0}(t)\}} \prod_{k \leq t} \mu_{p_0}(k) |\tilde{\Psi}\rangle\|^2 = \langle \tilde{\Psi} | \prod_t E_{\{s_{p_0}(t)\}} \prod_{k \leq t} \mu_{p_0}(k) |\tilde{\Psi}\rangle. \end{aligned} \quad (\text{S19})$$

Here  $\|\cdot\|^2$  denotes the state norm. First, note that this expression is a well-defined joint probability for the  $s_{p_0}(t)$  variables.  $P(\{s_{p_0}(t)\}|\{c_0^*(t)\})$  is always non-negative, and it is normalized as  $\sum_{\{s_{p_0}(t)\}} P(\{s_{p_0}(t)\}|\{c_0^*(t)\}) = 1$ , which could be verified by applying the normalization of POVM operators  $\sum_{\{s_{p_0}\}} E_{\{s_{p_0}\}} = I$  for each time slice. Besides, we can check that it is the true probability of syndrome measurements on the physical level. For example, imagine we are performing error correction in real world. At the time  $t'$ , we ask what is the syndrome measurement probability for the current step. Eq. (S19) tells us that it should be a probability at the  $t'$  step conditioned on the configurations of previous steps

$$\begin{aligned} P(\{s_{p_0}(t=t')\}|\{s_{p_0}(t < t')\}, \{c_0^*(t)\}) &= \frac{\sum_{\{s_{p_0}(t > t')\}} P(\{s_{p_0}(t)\}|\{c_0^*(t)\})}{\sum_{\{s_{p_0}(t \geq t')\}} P(\{s_{p_0}(t)\}|\{c_0^*(t)\})} = \frac{\|\prod_{t \leq t'} M_{\{s_{p_0}(t)\}} X_{c_0^*}^*(t) |\tilde{\Psi}\rangle\|^2}{\|\prod_{t < t'} M_{\{s_{p_0}(t)\}} X_{c_0^*}^*(t) |\tilde{\Psi}\rangle\|^2} \\ &= \frac{\text{tr}(E_{\{s_{p_0}(t')\}} \rho)}{\text{tr}(\rho)}, \quad \rho = \left( X_{c_0^*}^*(t') \prod_{t < t'} M_{\{s_{p_0}(t)\}} X_{c_0^*}^*(t) \right) |\tilde{\Psi}\rangle \langle \tilde{\Psi}| \left( X_{c_0^*}^*(t') \prod_{t < t'} M_{\{s_{p_0}(t)\}} X_{c_0^*}^*(t) \right)^\dagger. \end{aligned} \quad (\text{S20})$$

We arrive at the actual POVM probability at the current error correction step. Note that it also does not depend on

the Pauli errors after time  $t'$ . Calculate the expression in Eq. (S19) explicitly, we have

$$\begin{aligned} P(\{s_{p_0}(t)\}|\{c_0^*(t)\}) &= \frac{1}{\mathcal{Z}_{\{+\}} \sum_{\{\sigma_{e_0}\}} e^{\beta_0 \sum_{p_0} b_{p_0}} \prod_{p_0, t} \frac{\exp(\beta b_{p_0} s_{p_0}(t) \prod_{k \leq t} \mu_{p_0}(k))}{2 \cosh \beta}} \\ &= \frac{1}{\mathcal{Z}_{\{+\}} (2 \cosh \beta)^{NT}} \sum_{\{\sigma_{e_0}\}} \exp \left[ \sum_{p_0} b_{p_0} \left( \beta_0 + \beta \sum_t s_{p_0}(t) \prod_{k \leq t} \mu_{p_0}(k) \right) \right]. \end{aligned} \quad (\text{S21})$$

Here  $\mathcal{Z}_{\{+\}} = 4^N (\cosh^N \beta_0 + \sinh^N \beta_0)$  is the partition function of 2-d  $\mathbb{Z}_2$  lattice gauge theory. The  $\sigma_{e_0}$ 's have the same origin as Eq. (S2) through expansion under computational basis. Note that the above expression is independent of the choice of  $|\tilde{\Psi}\rangle$  in code space. This can be shown by expanding  $|\tilde{\Psi}\rangle$  under logical basis  $|\tilde{\Psi}\rangle = \Psi_{++} |++\rangle + \Psi_{+-} |+-\rangle + \Psi_{-+} |-+\rangle + \Psi_{--} |--\rangle$  and using Elitzur's theorem. Since the POVM operators  $E_{s_{p_0}(t)}$  at different times and different plaquettes are all complete and commute with each other, we may view the above probability as a joint probability of syndrome outcomes at different spacetime points, and it is conditioned on the error configuration. Notice that the syndromes at different times are correlated by the physical spin  $\sigma_{e_0}$ . That is because the imperfect measurement at each time step alters the instant quantum state, which affects the syndrome probability at the next time step. We can also construct a joint probability for both syndrome outcomes and error configuration. Noticing that the probability of a given error configuration is

$$P(\{c_0^*(t)\}) = \prod_{e_0, t} q^{\frac{1+\eta_{e_0}(t)}{2}} (1-q)^{\frac{1-\eta_{e_0}(t)}{2}} = \prod_{e_0, t} \frac{\exp(K \eta_{e_0}(t))}{2 \cosh K}, \quad (\text{S22})$$

we have

$$\begin{aligned} P(\{s_{p_0}(t)\}, \{c_0^*(t)\}) &= P(\{s_{p_0}(t)\}|\{c_0^*(t)\}) P(\{c_0^*(t)\}) \\ &= \frac{1}{\mathcal{Z}_{\{+\}} \prod_{e_0, t} \frac{\exp(K \eta_{e_0}(t))}{2 \cosh K}} \sum_{\{\sigma_{e_0}\}} e^{\beta_0 \sum_{p_0} b_{p_0}} \prod_{p, t} \frac{\exp(\beta b_{p_0} s_{p_0}(t) \prod_{k \leq t} \prod_{e_0 \in \partial p_0} \eta_{e_0}(k))}{2 \cosh \beta} \\ &= \frac{1}{\mathcal{Z}_{\{+\}} (2 \cosh \beta)^{NT} (2 \cosh K)^{2NT}} \sum_{\{\sigma_{e_0}\}} \exp \left[ K \sum_{e_0, t} \eta_{e_0}(t) + \sum_{p_0} b_{p_0} \left( \beta_0 + \beta \sum_t s_{p_0}(t) \prod_{k \leq t} \prod_{e_0 \in \partial p_0} \eta_{e_0}(k) \right) \right] \\ &\equiv P(\{s_{p_0}(t)\}, \{\eta_{e_0}(t)\}). \end{aligned} \quad (\text{S23})$$

Here  $K = -\frac{1}{2} \ln \frac{q}{1-q}$  and  $\eta_{e_0}(t) = \pm 1$  signs the presence of Pauli error, which means  $\eta_{e_0}(t) = -1$  if the error configuration  $\{c_0^*(t)\}$  includes edge  $e_0$  at time  $t$  and  $\eta_{e_0}(t) = +1$  otherwise. Besides the boundary configuration of an error chain  $c_0^*(t)$  can also be represented by  $\eta_{e_0}(t)$ , that is  $\mu_{p_0}(t) = \prod_{e_0 \in \partial p_0} \eta_{e_0}(t)$ .

Then we shall discuss in detail how could we decode with the syndrome outcomes  $\{s_{p_0}(t)\}$ . We mainly follow the method used in Ref. [5]. It is convenient to consider the situation that our logical information is stored forever. We extend the initial time  $t = 1$  to  $-\infty$  and the final time  $t = T$  to  $+\infty$ , which means that the syndrome measurement procedure is performed forever without beginning or end. The error correction procedure is represented as a 3 dimensional lattice in Fig. S4. The vertical plaquettes represent physical qubits at different times and the horizontal plaquettes mark syndrome outcomes. The Pauli  $X$  errors are associated with vertical plaquettes (horizontal dashed lines), and the measurement errors are associated with horizontal plaquettes (vertical dashed lines). A given syndrome forms a chain in 3-d spacetime, and we denote the syndrome chain as  $c_S^*$ . Note that  $c_S^*$  is a set of spacetime plaquettes, and we view it as a chain on the dual lattice (dashed lines in Fig. S4). We can also view it as a  $\mathbb{Z}_2$  valued vector with all the plaquettes as its basis. The task of the decoder is to find out both measurement errors and Pauli errors with respect to the information of syndrome  $c_S^*$ . Denote the error chain of both measurement and Pauli errors as  $c_E^*$ , it obvious that  $c_E^*$  should have the same boundary as  $c_S^*$ ,  $\partial^* c_S^* = \partial^* c_E^*$ . Here  $\partial^* c_S^*$  is the set of cubics where the boundary points of  $c_S^*$  lie in. Suppose the error chain decided by the decoder is  $c_{E'}^*$ , when  $c_{E'}^*$  and  $c_E^*$  are homologically equivalent, which means  $c_{E'}^* + c_E^*$  forms contractible loop (here the plus is defined mod  $\mathbb{Z}_2$ ), it should make no difference when we finally apply correction operator at  $t = +\infty$ , hence the error correction will be successful. But if  $c_{E'}^* + c_E^*$  forms contractible loops, then the corresponding correction operator will be containing logical  $X$  operator which has a nontrivial influence on logical information. In that case, the error correction will fail. So the task of the optimal decoder, named as maximum likelihood decoder, is to identify the equivalent class of error chains with the largest probability. Here the equivalent class of an error chain  $[c_E^*]$  is defined as the set of all error chains

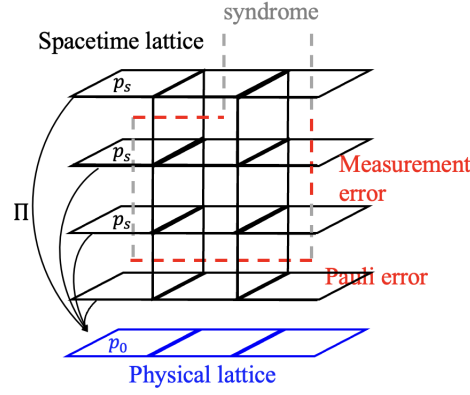

FIG. S4. 3-d spacetime of error history. The black lattice is the spacetime lattice, which takes periodic boundary condition at space directions and infinite boundary condition at time direction. The Pauli errors, measurement errors and error syndrome are represented as strings on the dual lattice (dashed lines). The horizontal red strings crossing timelike (vertical) plaquettes represent the locations of Pauli  $X$  errors which actually act on the physical lattice (blue). The vertical gray strings crossing spacelike (horizontal) plaquettes represent the error syndrome, which marks the locations of measurement results  $s_{p_0}(t) = -1$  at different time steps. The vertical red strings are where error syndromes do not match the Pauli errors that actually occurred, which we view as measurement errors.  $\Pi$  denotes the projection from the 3-d spacetime lattice to the 2-d physical lattice.

that are homologically equivalent to  $c_E^*$ .

The probability of error chain class could be derived from Eq. (S23). Notice that measurement error configuration can be inferred from the syndrome at that moment and error configuration in the past

$$\eta_{p_0}(t) = s_{p_0}(t) \prod_{k \leq t} \mu_{p_0}(k) = s_{p_0}(t) \prod_{k \leq t} \prod_{e_0 \in \partial p_0} \eta_{e_0}(k). \quad (\text{S24})$$

Substitute the above equation into Eq. (S23), we obtain the joint probability of both measurement and Pauli error

$$P(\{\eta_{p_0}(t)\}, \{\eta_{e_0}(t)\}) = \frac{1}{\mathcal{Z}_{\{+\}} \prod_t [(2 \cosh \beta)^N (2 \cosh K)^{2N}]} \times \sum_{\{\sigma_{e_0}\}} \exp \left[ K \sum_{e,t} \eta_{e_0}(t) + \sum_{p_0} b_{p_0} \left( \beta_0 + \beta \sum_t \eta_{p_0}(t) \right) \right]. \quad (\text{S25})$$

In this expression, we see that measurement errors at different time steps are correlated. Generally, the presence of measurement error increases the probability of measurement error at later times. We reinterpret the above equation on the 3-d lattice. Given an error chain in 3-d spacetime  $c_E^*$ , we still mark the location of error as  $\eta_p = -1$ . Specifically, measurement error at a spacelike plaquette is denoted as  $\eta_{p_s} = -1$ . Pauli error at a timelike plaquette is denoted as  $\eta_{p_t} = -1$ . Then the probability of the error chain is expressed as

$$P(c_E^*) = P(\{\eta_p\}) = \frac{1}{\mathcal{Z}_{\{+\}} \prod_t [(2 \cosh \beta)^N (2 \cosh K)^{2N}]} \times \sum_{\{\sigma_{e_0}\}} \exp \left[ K \sum_{p_t} \eta_{p_t} + \beta_0 \sum_{p_0} b_{p_0} + \beta \sum_{p_s} b_{\Pi(p_s)} \eta_{p_s} \right]. \quad (\text{S26})$$

Note that  $\sigma_{e_0}$ 's and associated  $b_{p_0}$ 's are viewed as lying on a 2-d lattice distinct from the 3-d spacetime representing error correction history. Each  $p_s$  is associated with an  $b_{\Pi(p_s)}$  on the 2-d physical lattice such that  $p_s$  and  $\Pi(p_s)$  correspond to the same space point as in Fig. S4.

The probability of error class  $[c_E]$  is calculated as a summation of probabilities of error chains that belong to the same equivalent class:

$$P([c_E]) = \sum_{c \in [c_E]} P(c) \quad (\text{S27})$$

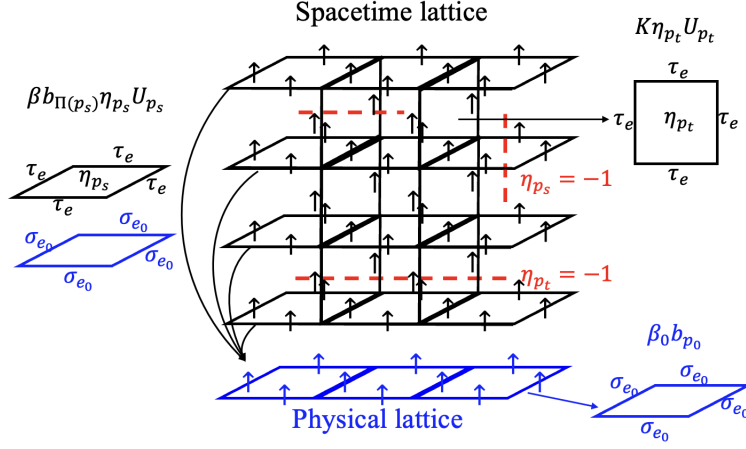

FIG. S5. Illustration of the SM model we obtained. The  $\tau_e$  spins are defined on the edges of 3-d spacetime lattice and the  $\sigma_{e_0}$ . There are three types of interactions in this model.  $\beta_0 b_{p_0}$  is the gauge interaction term defined on the physical lattice.  $K \eta_{p_t} U_{p_t}$  is the timelike gauge interaction on spacetime lattice. The  $\beta b_{\Pi(p_s)} \eta_{p_s} U_{p_s}$  term couples the spacelike gauge interaction term  $U_{p_s}$  to the gauge interaction term  $b_{\Pi(p_s)}$  on physical lattice. The  $\eta_p$ 's set the signs of gauge interactions on the spacetime lattice.

This summation can be done by introducing virtual spin  $\tau_p = \pm 1$  associated with each spacetime plaquette and relating it to each edge through  $\mathbb{Z}_2$  gauge interaction [5], as in Fig. S5. The summation of homologically equivalent error chains yields the same result as the summation of configurations of virtual spins  $\tau_e$  defined on edges up to a factor counting the number of 1-form symmetry operations since the sign changing of  $\tau_e$  corresponds to a deformation of error chain (see Fig. S6) and thus relates homologically equivalent error chains.:

$$\begin{aligned}
 P([c_E]) &= \frac{1}{\mathcal{N}_1} \sum_{\{\tau_p\}} P(\{\eta_p \prod_{e \in \partial p} \tau_e\}) \\
 &= \frac{1}{\mathcal{N}_1 \mathcal{Z}_{\{+\}} \prod_t [(2 \cosh \beta)^N (2 \cosh K)^{2N}]} \\
 &\times \sum_{\{\sigma_{e_0}\}, \{\tau_e\}} \exp \left[ \beta_0 \sum_{p_0} b_{p_0} + \beta \sum_{p_s} \left( b_{\Pi(p_s)} \eta_{p_s} \prod_{e \in \partial p_s} \tau_e \right) + K \sum_{p_t} \left( \eta_{p_t} \prod_{e \in \partial p_t} \tau_e \right) \right].
 \end{aligned} \tag{S28}$$

Here  $\mathcal{N}_1$  denotes the number of 1-form symmetry operations and it diverges for infinite time  $T$ . We now arrive at an SM model including both virtual spins  $\{\tau_p\}$  on the 3-d spacetime lattice and physical spins  $\{\sigma_{e_0}\}$  on a distinct 2-d space lattice. The virtual spins in this SM model describe the fluctuation of error chains in the same class. The physical spins are coupled to virtual spins on time-like plaquettes at all times since the probability of measurement errors at a certain time depends on the entire syndrome measurement history. The optimal decoding algorithm should select the error class  $[c_E]$  with the largest  $P([c_E])$ . Moreover, if the interaction configuration  $\{\eta_e\}$  is viewed as disordered with a correlated probability distribution  $P(\{\eta_e\})$  defined in equation S26, then the deconfinement-confinement phase transition point of virtual spins  $\{\tau_p\}$  in this disordered SM model should signify the error threshold of the error correction protocol as discussed in Ref. [5]. In summary, the quenched disordered SM model describing the error threshold is

$$\begin{aligned}
 \mathcal{Z}(\{\eta_p\}) &= \sum_{\{\sigma_{e_0}\}, \{\tau_e\}} \exp \left[ \beta_0 \sum_{p_0} b_{p_0} + \beta \sum_{p_s} b_{\Pi(p_s)} \eta_{p_s} U_{p_s} + K \sum_{p_t} \eta_{p_t} U_{p_t} \right], \\
 U_p &= \prod_{e \in \partial p} \tau_e, \quad b_{p_0} = \prod_{e_0 \in \partial p_0} \sigma_{e_0}, \\
 P(\{\eta_e\}) &= \frac{\sum_{\{\sigma_{e_0}\}} \exp \left[ \beta_0 \sum_{p_0} b_{p_0} + \beta \sum_{p_s} b_{\Pi(p_s)} \eta_{p_s} + K \sum_{p_t} \eta_{p_t} \right]}{\mathcal{Z}_{\{+\}} \prod_t [(2 \cosh \beta)^N (2 \cosh K)^{2N}]}.
 \end{aligned} \tag{S29}$$

Note that in our SM model, all the spacelike plaquettes are coupled with the  $\sigma_{e_0}$ 's, causing a highly non-local corre-

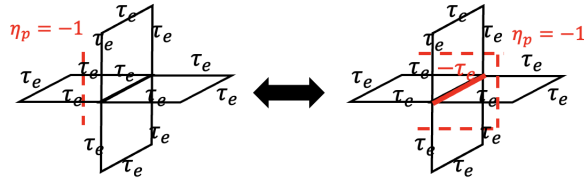

FIG. S6. Example of local symmetry. The red dashed lines represent the position where  $\eta_p = -1$ . The two  $\{\eta_p\}$  configurations yield the same partition function by redefining the spin colored red. Pictorially, flipping  $\tau_e$  spins is equivalent to a deformation of error chain.

lation in the timelike direction. This is a consequence of the imperfect measurement in the initial state preparation. When the initial state is well prepared  $\beta_0 \rightarrow +\infty$ , all the  $b_{p_0}$ 's will be set to +1 in Eq. (S29) and we arrive at a random plaquette gauge model:

$$\begin{aligned} \mathcal{Z}(\{\eta_p\}) &= \sum_{\{\sigma_{e_0}\}, \{\tau_e\}} \exp \left[ \beta \sum_{p_s} \eta_{p_s} U_{p_s} + K \sum_{p_t} \eta_{p_t} U_{p_t} \right], \\ U_p &= \prod_{e \in \partial p} \tau_e, \\ P(\{\eta_e\}) &= \frac{\exp \left[ K \sum_{p_t} \eta_{p_t} + \beta \sum_{p_s} \eta_{p_s} \right]}{\prod_t [(2 \cosh \beta)^N (2 \cosh K)^{2N}]}, \end{aligned} \quad (\text{S30})$$

which is derived in Ref. [5] to describe the error threshold under probabilistic measurement error.

From Eq. (S29) we can sum the  $\sigma_e$ 's out and arrive at the SM model containing pure  $\tau_e$  spins

$$\begin{aligned} \mathcal{Z}(\{\eta_p\}) &= \sum_{\{\tau_e\}} \left[ \prod_{p_0} \cosh(\beta_0 + \beta \sum_t \eta_{p_s} U_{p_s}) + \prod_{p_0} \sinh(\beta_0 + \beta \sum_t \eta_{p_s} U_{p_s}) \right] \exp \left[ K \sum_{p_t} \eta_{p_t} \right], \\ P(\{\eta_e\}) &= \frac{1}{[(\cosh \beta_0)^N + (\sinh \beta_0)^N] \prod_t [(2 \cosh \beta)^N (2 \cosh K)^{2N}]} \\ &\times \left[ \prod_{p_0} \cosh(\beta_0 + \beta \sum_t \eta_{p_s}) + \prod_{p_0} \sinh(\beta_0 + \beta \sum_t \eta_{p_s}) \right] \exp \left[ K \sum_{p_t} \eta_{p_t} \right]. \end{aligned} \quad (\text{S31})$$

### SIII. LOCAL SYMMETRY ON NISHIMORI LINE

The SM model  $\mathcal{Z}(\{\eta_p\})$  has a local symmetry when redefining the interaction background  $\{\eta_p\}$

$$\eta_p \rightarrow \eta_p \prod_{e \in \partial p} \nu_e, \quad \tau_e \rightarrow \tau_e \nu_e, \quad \nu_e = \pm 1. \quad (\text{S32})$$

as in Fig. S6. More precisely, the partition function is invariant under redefinition of background interaction configuration  $\{\eta_p\}$ :

$$\mathcal{Z}(\{\eta_p \prod_{e \in \partial p} \nu_e\}) = \mathcal{Z}(\{\eta_p\}) \quad (\text{S33})$$

since the influence is absorbed in the summation of spin configuration by redefining spin variable  $\tau'_e = \tau_e \nu_e$ . Note that  $\{\eta_p\}$  correspond to a representative error chain in error class  $[c_E]$ , and the local invariance Eq. (S32) tells us that  $\mathcal{Z}(\{\eta_p\})$  does not depend on the choice of representative error chain. It only depends on the homological class of error chain.

We will use the local invariance S32 on Nishimori line to derive several results about the phase structure [6, 7]. Under the presence of disorder, to compute an expectation value, we should first take the ensemble average for a particular interaction configuration (denoted by  $\langle \cdot \rangle_{\{\eta_p\}}$ ) and then take the disorder average on different configurations (denoted

as  $[\cdot]$ ). For a given observable  $O(\{\eta_p\}, \{\sigma_{e_0}\}, \{\tau_e\})$  depending on the  $\sigma$  spins,  $\tau$  spins and interaction configuration, these two kinds of averages are defined as:

$$\begin{aligned} \langle O \rangle_{\{\eta_p\}} &= \frac{1}{\mathcal{Z}(\{\eta_p\})} \sum_{\{\sigma_{e_0}\}, \{\tau_e\}} O \exp \left[ \beta_0 \sum_{p_0} b_{p_0} + \beta \sum_{p_s} b_{\Pi(p_s)} \eta_{p_s} U_{p_s} + K \sum_{p_t} \eta_{p_t} U_{p_t} \right] \\ [\langle O \rangle_{\{\eta_p\}}] &= \sum_{\{\eta_p\}} P(\{\eta_p\}) \langle O \rangle_{\{\eta_p\}} \end{aligned} \quad (\text{S34})$$

If an observable  $O(\{\eta_p\}, \{\sigma_{e_0}\}, \{\tau_e\})$  is also invariant under local symmetry transformation in Eq. (S32):

$$O(\{\eta_p \prod_{e \in \partial p} \nu_e\}, \{\sigma_{e_0}\}, \{\tau_e \nu_e\}) = O(\{\eta_p\}, \{\sigma_{e_0}\}, \{\tau_e\}) \quad (\text{S35})$$

then the expectation value can be evaluated as:

$$\begin{aligned} [\langle O \rangle] &= \sum_{\{\eta_p\}} \frac{P(\{\eta_p\})}{\mathcal{Z}(\{\eta_p\})} \sum_{\{\sigma_{e_0}\}, \{\tau_e\}} O(\{\eta_p\}, \{\sigma_{e_0}\}, \{\tau_e\}) \\ &\times \exp \left[ \beta_0 \sum_{p_0} b_{p_0} + \beta \sum_{p_s} b_{\Pi(p_s)} \eta_{p_s} U_{p_s} + K \sum_{p_t} \eta_{p_t} U_{p_t} \right] \\ &= \sum_{\{\eta_p\}} \frac{P(\{\eta_p \prod_{e \in \partial p} \nu_e\})}{\mathcal{Z}(\{\eta_p \prod_{e \in \partial p} \nu_e\})} \sum_{\{\sigma_{e_0}\}, \{\tau_e\}} O(\{\eta_p \prod_{e \in \partial p} \nu_e\}, \{\sigma_{e_0}\}, \{\tau_e\}) \\ &\times \exp \left[ \beta_0 \sum_{p_0} b_{p_0} + \beta \sum_{p_s} b_{\Pi(p_s)} \eta_{p_s} U_{p_s} \prod_{e \in \partial p_s} \nu_e + K \sum_{p_t} \eta_{p_t} U_{p_t} \prod_{e \in \partial p_t} \nu_e \right] \\ &= \sum_{\{\eta_p\}} \frac{P(\{\eta_p \prod_{e \in \partial p} \nu_e\})}{\mathcal{Z}(\{\eta_p\})} \sum_{\{\sigma_{e_0}\}, \{\tau_e\}} O(\{\eta_p\}, \{\sigma_{e_0}\}, \{\tau_e\}) \\ &\times \exp \left[ \beta_0 \sum_{p_0} b_{p_0} + \beta \sum_{p_s} b_{\Pi(p_s)} \eta_{p_s} U_{p_s} + K \sum_{p_t} \eta_{p_t} U_{p_t} \right] \\ &= \frac{1}{2^{3NT}} \sum_{\{\nu_e\}} \sum_{\{\eta_p\}} \frac{P(\{\eta_p \prod_{e \in \partial p} \nu_e\})}{\mathcal{Z}(\{\eta_p\})} \sum_{\{\sigma_{e_0}\}, \{\tau_e\}} O(\{\eta_p\}, \{\sigma_{e_0}\}, \{\tau_e\}) \\ &\times \exp \left[ \beta_0 \sum_{p_0} b_{p_0} + \beta \sum_{p_s} b_{\Pi(p_s)} \eta_{p_s} U_{p_s} + K \sum_{p_t} \eta_{p_t} U_{p_t} \right] \\ &= \frac{1}{2^{3NT} \mathcal{Z}_{\{+\}} (2 \cosh \beta)^{NT} (2 \cosh K)^{2NT}} \sum_{\{\sigma_{e_0}\}, \{\tau_e\}, \{\eta_p\}} O(\{\eta_p\}, \{\sigma_{e_0}\}, \{\tau_e\}) \\ &\times \exp \left[ \beta_0 \sum_{p_0} b_{p_0} + \beta \sum_{p_s} b_{\Pi(p_s)} \eta_{p_s} U_{p_s} + K \sum_{p_t} \eta_{p_t} U_{p_t} \right] \end{aligned} \quad (\text{S36})$$

In the third equality, we make use of the local symmetry. In the fourth equality we averaged over different  $\{\nu_e\}$  since the final result  $[\langle O \rangle]$  is independent of  $\{\nu_e\}$ . The fifth equality is obtained by noticing that:

$$\sum_{\{\nu_e\}} P(\{\eta_p \prod_{e \in \partial p} \nu_e\}) = \frac{\mathcal{Z}(\{\eta_p\})}{\mathcal{Z}_{\{+\}} (2 \cosh \beta)^{NT} (2 \cosh K)^{2NT}} \quad (\text{S37})$$

First we consider  $O = W_{A_0} = \prod_{p_0 \in A_0} b_{p_0}$  which is the Wilson loop on 2-d physical lattice. Clearly, it satisfies Eq.

(S35). So we calculate its expectation value as:

$$\begin{aligned}
\langle W_{A_0} \rangle &= \frac{1}{2^{3NT} \mathcal{Z}_{\{+\}} (2 \cosh \beta)^{NT} (2 \cosh K)^{2NT}} \\
&\quad \sum_{\{\sigma_{e_0}\}, \{\tau_e\}, \{\eta_p\}} W_{A_0} \exp \left[ \beta_0 \sum_{p_0} b_{p_0} + \beta \sum_{p_s} b_{\Pi(p_s)} \eta_{p_s} U_{p_s} + K \sum_{p_t} \eta_{p_t} U_{p_t} \right] \\
&= \frac{1}{\mathcal{Z}_{\{+\}} \sum_{\{\sigma_{e_0}\}}} W_{A_0} \exp \left[ \beta_0 \sum_{p_0} b_{p_0} \right] = \langle W_{A_0} \rangle_{\{+\}} \\
&= \frac{(\tanh \beta_0)^{|A_0|} + (\tanh \beta_0)^{N-|A_0|}}{1 + (\tanh \beta_0)^N}
\end{aligned} \tag{S38}$$

Here  $\langle \cdot \rangle_{\{+\}}$  denotes the expectation value for the pure 2-d  $\mathbb{Z}_2$  gauge theory of physical spins  $\sigma_{e_0}$ ,  $\mathcal{Z}_{\{+\}} = \sum_{\{\sigma_{e_0}\}} \exp \left[ \beta_0 \sum_{p_0} b_{p_0} \right]$ . Actually, the above derivation works for any observable contains purely  $\sigma_{e_0}$  spins. So we conclude that the  $\sigma_{e_0}$  spins in SM model shown in Eq. (S29) behaves exactly the same as pure 2-d  $\mathbb{Z}_2$  gauge theory. Specifically for the Wilson loop  $W_{A_0}$ , we find it obeys area law for any finite  $\beta_0$ , same as 2-d  $\mathbb{Z}_2$  lattice gauge theory, so the  $\sigma_{e_0}$  spins always stays in disordered phase.

We may also compute the internal energy, which is also invariant under the transformation shown in Eq. (S32). Given that

$$\begin{aligned}
\langle \eta_{p_s} b_{\pi(p_s)} U_{p_s} \rangle &= \frac{1}{2^{3NT} \mathcal{Z}_{\{+\}} (2 \cosh \beta)^{NT} (2 \cosh K)^{2NT}} \\
&\quad \times \sum_{\{\sigma_{e_0}\}, \{\tau_e\}, \{\eta_p\}} \eta_{p_s} b_{\pi(p_s)} U_{p_s} \exp \left[ \beta_0 \sum_{p_0} b_{p_0} + \beta \sum_{p_s} b_{\Pi(p_s)} \eta_{p_s} U_{p_s} + K \sum_{p_t} \eta_{p_t} U_{p_t} \right] \\
&= \frac{1}{2^{3NT} \mathcal{Z}_{\{+\}} (2 \cosh \beta)^{NT} (2 \cosh K)^{2NT}} \sum_{\{\sigma_{e_0}\}, \{\tau_e\}} (2 \sinh \beta) (2 \cosh \beta)^{NT-1} (2 \cosh K)^{2NT} \exp \left[ \beta_0 \sum_{p_0} b_{p_0} \right] \\
&= \tanh \beta,
\end{aligned} \tag{S39}$$

and similarly

$$\begin{aligned}
\langle \eta_{p_t} U_{p_t} \rangle &= \frac{1}{2^{3NT} \mathcal{Z}_{\{+\}} (2 \cosh \beta)^{NT} (2 \cosh K)^{2NT}} \\
&\quad \times \sum_{\{\sigma_{e_0}\}, \{\tau_e\}, \{\eta_p\}} \eta_{p_t} U_{p_t} \exp \left[ \beta_0 \sum_{p_0} b_{p_0} + \beta \sum_{p_s} b_{\Pi(p_s)} \eta_{p_s} U_{p_s} + K \sum_{p_t} \eta_{p_t} U_{p_t} \right] \\
&= \frac{1}{2^{3NT} \mathcal{Z}_{\{+\}} (2 \cosh \beta)^{NT} (2 \cosh K)^{2NT}} \sum_{\{\sigma_{e_0}\}, \{\tau_e\}} (2 \sinh K) (2 \cosh \beta)^{NT} (2 \cosh K)^{2NT-1} \exp \left[ \beta_0 \sum_{p_0} b_{p_0} \right] \\
&= \tanh K,
\end{aligned} \tag{S40}$$

we have the expression for internal energy

$$\begin{aligned}
\mathcal{U} &= \langle -\beta_0 \sum_{p_0} b_{p_0} - \beta \sum_{p_s} b_{\Pi(p_s)} \eta_{p_s} U_{p_s} - K \sum_{p_t} \eta_{p_t} U_{p_t} \rangle \\
&= -N \beta_0 \frac{\tanh \beta_0 + (\tanh \beta_0)^{N-1}}{1 + (\tanh \beta_0)^N} - NT \beta \tanh \beta - 2NT K \tanh K.
\end{aligned} \tag{S41}$$

Then consider the Wilson loop for  $\tau_e$  spins  $W_A = \prod_{p \in A} U_p = \prod_{e \in \partial A} \tau_e$ . Note that it is not invariant under Eq.

(S32). By a similar calculation as Eq. (S36) we have:

$$\begin{aligned}
[\langle W_A \rangle] &= \sum_{\{\eta_p\}} \frac{P(\{\eta_p\})}{\mathcal{Z}(\{\eta_p\})} \sum_{\{\sigma_{e_0}\}, \{\tau_e\}} W_A \exp \left[ \beta_0 \sum_{p_0} b_{p_0} + \beta \sum_{p_s} b_{\Pi(p_s)} \eta_{p_s} U_{p_s} + K \sum_{p_t} \eta_{p_t} U_{p_t} \right] \\
&= \sum_{\{\eta_p\}} \frac{P(\{\eta_p \prod_{e \in \partial p} \nu_e\})}{\mathcal{Z}(\{\eta_p\})} \sum_{\{\sigma_{e_0}\}, \{\tau_e\}} W_A \prod_{e \in \partial A} \nu_e \\
&\quad \times \exp \left[ \beta_0 \sum_{p_0} b_{p_0} + \beta \sum_{p_s} b_{\Pi(p_s)} \eta_{p_s} U_{p_s} + K \sum_{p_t} \eta_{p_t} U_{p_t} \right] \\
&= \frac{1}{2^{3NT}} \sum_{\{\nu_e\}} \sum_{\{\eta_p\}} \frac{P(\{\eta_p \prod_{e \in \partial p} \nu_e\}) \prod_{e \in \partial A} \nu_e}{\mathcal{Z}(\{\eta_p\})} \sum_{\{\sigma_{e_0}\}, \{\tau_e\}} W_A \\
&\quad \times \exp \left[ \beta_0 \sum_{p_0} b_{p_0} + \beta \sum_{p_s} b_{\Pi(p_s)} \eta_{p_s} U_{p_s} + K \sum_{p_t} \eta_{p_t} U_{p_t} \right] \\
&= \frac{1}{2^{3NT} \mathcal{Z}_{\{+\}} (2 \cosh \beta)^{NT} (2 \cosh K)^{2NT}} \sum_{\{\eta_p\}} \mathcal{Z}(\{\eta_p\}) \langle W_A \rangle^2 \\
&= [\langle W_A \rangle^2]
\end{aligned} \tag{S42}$$

The result  $[\langle W_A \rangle] = [\langle W_A \rangle^2]$  signifies the absence of gauge glass phase ( $[\langle W_A \rangle] = 0$ ,  $[\langle W_A \rangle^2] > 0$ ) on the Nishimori line [7].

In addition, one may find that the modified Wilson loop  $W_A \prod_{p \in A} \eta_p$  is invariant under local symmetry. It can be calculated as

$$\begin{aligned}
[\langle W_A \prod_{p \in A} \eta_p \rangle] &= \frac{1}{2^{3NT} \mathcal{Z}_{\{+\}} (2 \cosh \beta)^{NT} (2 \cosh K)^{2NT}} \\
&\quad \times \sum_{\{\sigma_{e_0}\}, \{\tau_e\}, \{\eta_p\}} W_A \prod_{p \in A} \eta_p \exp \left[ \beta_0 \sum_{p_0} b_{p_0} + \beta \sum_{p_s} b_{\Pi(p_s)} \eta_{p_s} U_{p_s} + K \sum_{p_t} \eta_{p_t} U_{p_t} \right] \\
&= \frac{1}{2^{3NT} \mathcal{Z}_{\{+\}} (2 \cosh \beta)^{NT} (2 \cosh K)^{2NT}} \sum_{\{\sigma_{e_0}\}, \{\tau_e\}} \exp \left[ \beta_0 \sum_{p_0} b_{p_0} \right] \\
&\quad \times \left( \prod_{p_s \in A_s} \sum_{\eta_{p_s}} \eta_{p_s} U_{p_s} \exp [\beta b_{\Pi(p_s)} \eta_{p_s} U_{p_s}] \prod_{p_s \notin A_s} \sum_{\eta_{p_s}} \exp [\beta b_{\Pi(p_s)} \eta_{p_s} U_{p_s}] \right) \\
&\quad \times \left( \prod_{p_t \in A_t} \sum_{\eta_{p_t}} \eta_{p_t} U_{p_t} \exp [K \eta_{p_t} U_{p_t}] \prod_{p_t \notin A_t} \sum_{\eta_{p_t}} \exp [K \eta_{p_t} U_{p_t}] \right) \\
&= \frac{1}{2^{3NT} \mathcal{Z}_{\{+\}} (2 \cosh \beta)^{NT} (2 \cosh K)^{2NT}} \sum_{\{\sigma_{e_0}\}, \{\tau_e\}} \exp \left[ \beta_0 \sum_{p_0} b_{p_0} \right] \\
&\quad \times \left( \prod_{p_s \in A_s} b_{\pi(p_s)} \right) (2 \sinh \beta)^{|A_s|} (2 \cosh \beta)^{NT - |A_s|} (2 \sinh K)^{|A_t|} (2 \cosh K)^{2NT - |A_t|} \\
&\quad \langle W_{\Pi(A)} \rangle_{\{+\}} (\tanh \beta)^{|A_s|} (\tanh K)^{|A_t|}
\end{aligned} \tag{S43}$$

Here  $A_s$  and  $A_t$  denote the sets of spacelike plaquettes and timelike plaquettes contained in  $A$  respectively.  $\Pi$  is the projection onto physical lattice, see Fig. S9. This expression reveals that  $\tau_e$ 's and  $\sigma_e$ 's are correlated and their Wilson loops somehow depend on each other. However, the modified Wilson loop  $W_A \prod_{p \in A} \eta_p$  cannot serve as the correct order parameter for the error threshold.

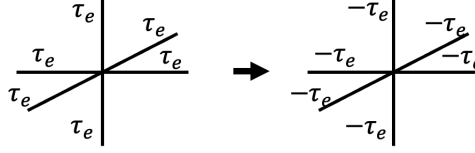

FIG. S7. Example of 1-form symmetry operation. The  $\tau_e$  spins on a closed surface (surrounding the center vertex in this figure) are flipped.

#### SIV. LOW TEMPERATURE EXPANSION

The ordered (deconfinement) phase is expected to exist at the exact zero temperature point (on the Nishimori line)  $\beta_0, \beta, K \rightarrow +\infty$ . Near the zero temperature point, we may perform a low-temperature expansion for Wilson loops to show if the ordered phase still persists to some finite temperature. Assume  $e^{-\beta_0}$ ,  $e^{-\beta}$ ,  $e^{-K}$  are of the same order, we expand  $[\langle W_A \rangle]$  up to the order  $e^{-4\beta}$  following the method discussed in Ref. [3].

We first perform the expansion for the disorder probability  $P(\{\eta_p\})$ . Through the expression of  $P(\{\eta_p\})$

$$P(\{\eta_p\}) = \frac{2^{N+1} \sum_{\{b_{p_0}\}} \frac{1+\prod_{p_0} b_{p_0}}{2} \exp \left[ \beta_0 \sum_{p_0} b_{p_0} + \beta \sum_{p_s} b_{\Pi(p_s)} \eta_{p_s} + K \sum_{p_t} \eta_{p_t} \right]}{\mathcal{Z}_{\{+\}} \prod_t [(2 \cosh \beta)^N (2 \cosh K)^{2N}]}. \quad (\text{S44})$$

We notice that the zeroth order is contributed by the configuration that all  $b_{p_0}$  and  $\eta_p$  are equal to +1. The order  $e^{-2\beta}$  is given by flipping one of the  $\eta_{p_s}$  to -1. The order  $e^{-4\beta}$  is given by flipping any two of the  $\eta_{p_s}$  or flipping two of  $b_{p_0}$ s. Note that the parity of  $\{b_{p_0}\}$  configuration must be even. Then we find that the numerator is expanded as

$$2^{N+1} E^{N\beta_0 + NT\beta + 2NTK} \left[ \delta_{\{+\}} + e^{-2K} \sum_{p_t} \delta_{\{p_t\}} + e^{-2\beta} \sum_{p_s} \delta_{\{p_s\}} \right. \\ \left. + e^{-4K} \sum_{(p_t, p'_t)} \delta_{\{(p_t, p'_t)\}} + e^{-4\beta} \sum_{(p_s, p'_s)} \delta_{\{(p_s, p'_s)\}} + e^{-2\beta-2K} \sum_{(p_s, p_t)} \delta_{\{(p_s, p_t)\}} + e^{-4\beta_0} \sum_{(p_0, p'_0)} \delta_{\{\Pi^{-1}(p_0, p'_0)\}} \right]. \quad (\text{S45})$$

Here  $(p, p')$  denotes a pair of different plaquettes. For example  $(p_s, p'_s)$  denotes a pair of spacelike plaquettes and the summation  $\sum_{(p_s, p'_s)}$  is taken on all such pairs. We have used a simplified notation for the Kronecker delta symbol.  $\delta_+$  means that all the  $\eta_{p_s}$  are fixed to be +1,  $\delta_+ = \prod_p \delta_{\eta_p, +}$ .  $\delta_p$  denotes that  $\eta_p$  on the given plaquette  $p$  is flipped to -1,  $\delta_p = \delta_{\eta_p, -} \prod_{p' \neq p} \delta_{\eta_{p'}, +}$ , and similar for  $\delta_{(p, p')}$ ,  $\delta_{(p, p')} = \delta_{\eta_p, -} \delta_{\eta_{p'}, -} \prod_{p'' \neq p, p'} \delta_{\eta_{p''}, +}$ . Finally  $\delta_{\Pi^{-1}(p_0, p'_0)}$  means that all the spacelike plaquettes whose projection on the physical lattice is  $p_0$  or  $p'_0$  are set to be -1,  $\delta_{\Pi^{-1}(p_0, p'_0)} = \prod_{p_s | \Pi(p_s) = p_0} \delta_{\eta_{p_s}, -} \prod_{p'_s | \Pi(p'_s) = p'_0} \delta_{\eta_{p'_s}, -} \prod_{p''_s | \Pi(p''_s) \neq p_0, p'_0} \delta_{\eta_{p''_s}, +}$ . The number of integer times  $T$  should be sent to  $+\infty$  at the end of the calculation. Combined with the denominator, we arrive at a perturbative expression for disorder probability

$$P(\{\eta_p\}) \simeq [1 - (1 - 2NTe^{-2K} - NTe^{-2\beta}) (2NTe^{-2K} + NTe^{-2\beta}) \\ - \left( \binom{2NT}{2} e^{-4K} + \binom{NT}{2} e^{-4\beta} + 2(NT)^2 e^{-2K-2\beta} + \binom{N}{2} e^{-4\beta_0} \right) \delta_{\{+\}} \\ + (1 - 2NTe^{-2K} - NTe^{-2\beta}) \left[ e^{-2K} \sum_{p_t} \delta_{\{p_t\}} + e^{-2\beta} \sum_{p_s} \delta_{\{p_s\}} \right] \\ + e^{-4K} \sum_{(p_t, p'_t)} \delta_{\{(p_t, p'_t)\}} + e^{-4\beta} \sum_{(p_s, p'_s)} \delta_{\{(p_s, p'_s)\}} + e^{-2\beta-2K} \sum_{(p_s, p_t)} \delta_{\{(p_s, p_t)\}} + e^{-4\beta_0} \sum_{(p_0, p'_0)} \delta_{\{\Pi^{-1}(p_0, p'_0)\}}]. \quad (\text{S46})$$

Then we analyze the ensemble-averaged value for the interaction configurations that appeared in the above expression. Keeping in mind the fact that the interaction term  $U_p$  and Wilson loop  $W_A$  are both invariant under 1-form symmetry operations which flip the spins on a 2-d surface on the dual lattice as in Fig. S7, when performing the spin configuration summation for the lowest few orders we extract a factor of 1-form symmetry operation numbers  $\mathcal{N}_1$  and evaluate the coefficient for each order on an equivalent class of spin configurations module 1-form symmetry.

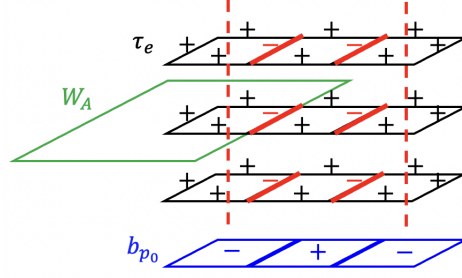

FIG. S8. Spin configuration when two  $b_{p_0}$  are flipped. The  $\{b_{p_0}\}$  configuration is shown on the blue lattice. The timelike plaquettes are omitted for explicitness. The two red dashed strings represent the locations of  $-1$  plaquette interaction caused by  $b_{\Pi(p_s)} = -1$ , and their energy cost can be eliminated by flipping the spins on the solid red edges.

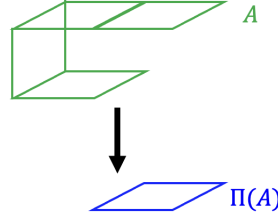

FIG. S9. The action of projection  $\Pi$  on surface  $A$ . The above surface lies inside 3-d spacetime and its projection on 2-d space is shown below. Their boundaries correspondingly are Wilson loops in 3-d spacetime and 2-d space.

First, consider the case all  $\eta_p = +1$ , and we want to compute

$$\langle W_A \rangle_{\{+\}} = \frac{1}{\mathcal{Z}(\{+\})} \sum_{\{\sigma_{e_0}\}, \{\tau_e\}} \left( \prod_{e \in \partial A} \tau_e \right) \exp \left[ \beta_0 \sum_{p_0} b_{p_0} + \beta \sum_{p_s} b_{\Pi(p_s)} U_{p_s} + K \sum_{p_t} U_{p_t} \right]. \quad (\text{S47})$$

The 0th order is contributed by the ground states, and a representative spin configuration is that all  $\tau_e = +1$  and  $b_{p_0} = +1$ . It leads to the term:

$$\mathcal{N}_1 2^{N+1} e^{N\beta_0 + NT\beta + 2NTK} \quad (\text{S48})$$

in both the numerator and denominator. Now if we flip one of the  $\tau_e$  spins to  $-1$ , it increases the energy of four neighbor plaquettes and results in a term of order  $e^{-8\beta}$ , which is not included in our expansion. However, if we flip two  $b_{p_0}$ s, this only yields a term of order  $e^{-4\beta_0}$  in the infinite boundary condition case. When two  $b_{p_0}$ s are flipped, it leads to  $-1$  interactions on two strings of spacelike plaquettes corresponding to the position of  $b_{p_0}$ , as shown in S8, and it should cost infinite energy. However, the energy cost can be eliminated by the local symmetry transformation in Eq. (S32). The two strings can be viewed as merged together by setting the  $\tau_e$  spins on the surface connecting them to  $-1$ . Deformation of the surface is nothing but a 1-form symmetry operation and has already been mod out. Combining both the  $b_{p_0}$  configuration and the  $\tau_e$  spin configuration, the total energy cost is just  $4\beta_0$ . Now consider the value of the Wilson loop. During the process of merging two strings together, if they cross the Wilson loop for odd times, then exactly one of the spins on the boundary of region  $A$  will be flipped to  $-1$ . So the value of the Wilson loop for that configuration is  $-1$ . But if the Wilson loop is crossed for even times, it still gets  $+1$ . The total contribution of order  $e^{-4\beta_0}$  is obtained by summing all the choices for flipping two  $b_{p_0}$ s, which contains  $\binom{N}{2}$  terms. By counting the number of odd time crosses, we obtain the expression for an additional term in the numerator

$$\left( \binom{N}{2} - 2|\Pi(A)|(N - |\Pi(A)|) \right) e^{-4\beta_0}. \quad (\text{S49})$$

Here we define  $\Pi(A)$  as the projection of region  $A$  on the spacelike 2-d lattice module  $\mathbb{Z}_2$ . The timelike plaquettes are dropped under projection, and an even number of spacelike plaquettes on the same space position also leads to zero, as in Fig. S9. For denominator, the new term is just  $\binom{N}{2} e^{-4\beta_0}$ . So the expansion of  $\langle W_A \rangle_{\{+\}}$  is evaluated as

$$\begin{aligned} \langle W_A \rangle_{\{+\}} &\simeq \frac{\mathcal{N}_1 2^{N+1} e^{N\beta_0 + NT\beta + 2NTK} \left[ 1 + \left( \binom{N}{2} - 2|\Pi(A)|(N - |\Pi(A)|) \right) e^{-4\beta_0} \right]}{\mathcal{N}_1 2^{N+1} e^{N\beta_0 + NT\beta + 2NTK} \left[ 1 + \binom{N}{2} e^{-4\beta_0} \right]} \\ &\simeq 1 - 2|\Pi(A)|(N - |\Pi(A)|) e^{-4\beta_0}. \end{aligned} \quad (\text{S50})$$

From this expression, we can roughly say that  $\langle W_A \rangle_{\{+\}}$  decays with respect to the spacelike area.

Now we evaluated the Wilson loop configurations that only one  $\eta_p$  is flipped. Suppose a timelike plaquette  $p_t$  is flipped. Now the ground state energy is  $2K$  higher than the previous all  $\eta_p = +1$  case and the ground state spin configuration remains the same, which is all  $\tau_e = +1$ . The lowest excitation is caused by flipping one of the spins at the boundary of  $p_t$ , which has the extra energy  $4K$ . It eventually results in terms of order  $e^{-4K}$ . Notice that the probability of  $\eta_{p_t} = -1$  is already of the order  $e^{-2K}$ , so we only need to concern about the ground state in our expansion, and it leads to

$$\langle W_A \rangle_{\{p_t\}} \simeq 1. \quad (\text{S51})$$

Similarly, for the spacelike plaquette flipping, we also have

$$\langle W_A \rangle_{\{p_s\}} \simeq 1. \quad (\text{S52})$$

Then we consider the configuration where two  $\eta_p$ s are flipped. Notice that only the ground state contribution survives in our expansion since the probability is already of the order  $e^{-4\beta}$ . We the two flipped  $\eta_p$ s do not contact each other, the representative spin configuration for ground state is still all  $\tau_e = +1$  and only those two plaquettes where  $\eta_p = -1$  have energy costs. But when the two flipped plaquettes are nearest neighbors, there will be two degenerate (ignoring the energetic difference between  $\beta$  and  $K$ ) configurations that both have energy costs on two plaquettes. They are distinguished by whether the contacting edge of the two plaquettes is flipped to  $-1$ . If the contacting edges lie on the Wilson loop, then summing the two degenerate configurations leads to  $W_A = 0$ . So assume the two flipped plaquettes are  $p$  and  $p'$ , then the Wilson loop takes the value

$$\langle W_A \rangle_{\{(p,p')\}} \simeq 1 - |\partial A \cap \partial p \cap \partial p'|. \quad (\text{S53})$$

If the two plaquettes and the Wilson loop intersect at one edge,  $|\partial A \cap \partial p \cap \partial p'|$  takes 1. Otherwise, it takes 0. Consider the disorder summation of these configurations. Each edge connects to 4 plaquettes, yielding 6 pairs of nearest-neighbor plaquettes. By noticing that each timelike edge is associated with 6 pairs of timelike plaquettes while each spacelike edge is associated with a pair of timelike plaquettes, a pair of spacelike plaquettes and 4 combinations of spacelike and timelike plaquettes, we find that

$$\begin{aligned} e^{-4\beta} \sum_{(p_s, p'_s)} \langle W_A \rangle_{\{(p_s, p'_s)\}} &\simeq e^{-4\beta} \left( \binom{NT}{2} - |\partial A|_s \right) \\ e^{-4K} \sum_{(p_t, p'_t)} \langle W_A \rangle_{\{(p_t, p'_t)\}} &\simeq e^{-4K} \left( \binom{2NT}{2} - |\partial A|_s - 6|\partial A|_t \right) \\ e^{-2\beta-2K} \sum_{(p_t, p_s)} \langle W_A \rangle_{\{(p_t, p_s)\}} &\simeq e^{-2\beta-2K} (2(NT)^2 - 4|\partial A|_s). \end{aligned} \quad (\text{S54})$$

Here  $|\partial A|_s$  denotes the number of spacelike edges in  $\partial A$  and  $|\partial A|_t$  is the number of timelike edges in  $\partial A$ .

Finally we turn to the configuration denoted as  $\{\Pi^{-1}(p_0, p'_0)\}$ , which means all the spacelike interactions  $\eta_{p_s}$  along the timelike strings with the same space position as  $p_0$  or  $p'_0$  are flipped. In this case, a similar argument while evaluating Eq. (S50) could be applied. The two timelike strings are merged together by setting the spins in the interval to  $-1$ , which gives us the ground state configuration. So the leading order of the Wilson loop is

$$\langle W_A \rangle_{\{\Pi^{-1}(p_0, p'_0)\}} \simeq \pm 1. \quad (\text{S55})$$

which takes  $-1$  when only one of the  $p_0$  and  $p'_0$  stays in  $\Pi(A)$  and takes  $+1$  otherwise. Performing the disorder summation, we find that

$$e^{-4\beta_0} \sum_{(p_0, p'_0)} \langle W_A \rangle_{\{\Pi^{-1}(p_0, p'_0)\}} \simeq e^{-4\beta_0} \left( \binom{N}{2} - 2|\Pi(A)|(N - |\Pi(A)|) \right). \quad (\text{S56})$$

Putting all these stuff together, we arrive at the low-temperature expansion for the Wilson loop

$$[\langle W_A \rangle] \simeq 1 - 4|\Pi(A)|(N - |\Pi(A)|)e^{-4\beta_0} - |\partial A|_s (e^{-4\beta} + e^{-4K} + 4e^{-2\beta-2K}) - 6|\partial A|_t e^{-4K} \\ \simeq \exp [-4|\Pi(A)|(N - |\Pi(A)|)e^{-4\beta_0} - |\partial A|_s (e^{-4\beta} + e^{-4K} + 4e^{-2\beta-2K}) - 6|\partial A|_t e^{-4K}]. \quad (\text{S57})$$

Note that the factor  $|\Pi(A)|(N - |\Pi(A)|)$  appears because our space manifold is a closed surface. The result is natural to be symmetric between  $\Pi(A)$  and the 2-d complement of  $\Pi(A)$ . We also notice that the number of integer time  $T$  automatically vanishes in these expressions so they already suit the case  $T \rightarrow +\infty$ .

From Eq. (S57) we can see that once the initial state preparation suffers from imperfect measurement, the scaling behavior of Wilson loops becomes anisotropic for space and time direction. For a Wilson loop  $A$  purely containing spacelike plaquettes, we have

$$[\langle W_A \rangle] \simeq \exp [-4|A|(N - |A|)e^{-4\beta_0} - |\partial A| (e^{-4\beta} + e^{-4K} + 4e^{-2\beta-2K})]. \quad (\text{S58})$$

For large enough  $N$  and large enough Wilson loop satisfying  $|A| < N/2$ , the area law decaying term dominates and the perimeter term can be ignored. So we conclude that the spacelike Wilson loop always decays with respect to the area at finite temperature even when the temperature is sufficiently low. Equivalently we can say that once the initial state is prepared under imperfect measurement, the spacelike Wilson loop always obeys area law. However, for a timelike Wilson loop, we will get:

$$[\langle W_A \rangle] \simeq \exp [- (e^{-4\beta} + e^{-4K} + 4e^{-2\beta-2K}) |\partial A|_s - 6e^{-4K} |\partial A|_t]. \quad (\text{S59})$$

so there will be a finite temperature phase for it to exhibit perimeter law scaling.

As we mentioned in the main text, the subtlety of Eq. (S57) is that we cannot directly take the thermodynamic limit  $N \rightarrow \infty$ . However, we may infer the thermodynamic result in analogy to the 2-d  $\mathbb{Z}_2$  gauge theory. We may expand the Wilson loop for 2-d  $\mathbb{Z}_2$  gauge theory Eq. (S38) also up to  $e^{-4\beta_0}$ :

$$\langle W_{A_0} \rangle_{\{+\}} \simeq 1 - 2|A_0|(N - |A_0|)e^{-4\beta_0}. \quad (\text{S60})$$

Compared with Eq. (S57) we find an approximate relation under low temperatures:

$$[\langle W_A \rangle] \simeq \langle W_{\Pi(A)} \rangle_{\{+\}}^2 \exp [-|\partial A|_s (e^{-4\beta} + e^{-4K} + 4e^{-2\beta-2K}) - 6|\partial A|_t e^{-4K}]. \quad (\text{S61})$$

In this expression  $[\langle W_A \rangle]$  is a Wilson loop for  $\tau_e$  spins and it relates to a Wilson loop  $\langle W_{\Pi(A)} \rangle_{\{+\}}$  for  $\sigma_{e_0}$  spins in the 2-d physical lattice. Recall that  $\langle \cdot \rangle_{\{+\}}$  denotes the expectation value for 2-d  $\mathbb{Z}_2$  gauge theory  $\mathcal{Z}_{\{+\}} = \sum_{\{\sigma_{e_0}\}} \exp(\beta_0 \sum_{p_0} b_{p_0})$ . The expression in Eq. (S61) absorbs the size of space  $N$  and we expect it to valid under the thermodynamic limit. Turn back to Eq. (S38). If we take the  $N \rightarrow +\infty$  limit first (keeping  $A_0$  a finite region) and then perform low-temperature expansion, we arrive at

$$\langle W_{A_0} \rangle_{\{+\}} \simeq 1 - 2|A_0|e^{-2\beta_0} + 2|A_0|^2 e^{-4\beta_0}. \quad (\text{S62})$$

The difference between Eq. (S60) and Eq. (S62) arise from the criticality at zero temperature  $\beta_0 = +\infty$ . The  $e^{-2\beta_0}$  term exhibit a discontinuity at zero temperature, which leads to the non-commuting of  $N \rightarrow +\infty$  limit and  $\beta_0 \rightarrow +\infty$  limit. A similar critical behavior should be found in  $[\langle W_A \rangle]$ . If the thermodynamic limit is taken before the low-temperature expansion, we infer that (not a rigorous proof)

$$[\langle W_A \rangle] \simeq \exp [-4|\Pi(A)|e^{-2\beta_0} + 4|\Pi(A)|^2 e^{-4\beta_0} - |\partial A|_s (e^{-4\beta} + e^{-4K} + 4e^{-2\beta-2K}) - 6|\partial A|_t e^{-4K}]. \quad (\text{S63})$$

In all, we expect that spacelike Wilson loops still decay with respect to area under the thermodynamic limit. Another way to think about the area law of spacelike Wilson loops when  $N \rightarrow +\infty$  is to reconsider an open boundary condition at the spacelike directions and take an infinitely large system size before calculating the low-temperature expansion. Then an odd number of flipped  $b_{p_0}$  is allowed since we can send one in a pair of  $b_{p_0}$ 's to the infinity and eliminate it. Thus up to the leading order we have  $[\langle W_A \rangle] \simeq \exp [-4|\Pi(A)|e^{-2\beta_0}]$ . Although this open boundary condition does not correspond to any QEC procedure, we expect that the phase structure of the SM model does not depend on the choice of spacelike boundary conditions, and the expectation values of the order parameter for both the two kinds of boundary conditions should match under the thermodynamic limit.

In addition, Eq. S61 implies that the area law behavior of spacelike Wilson loops is controlled by the finite temperature disordered phase of the 2-d physical  $\sigma_{e_0}$  spins. Note that the area law behavior of the Wilson loop

$\langle W_{A_0} \rangle_{\{+\}}$  is used in Ref. [1, 2] to argue the absence of long-range entanglement in the imperfect initial state. So in some sense, Eq. (S61) relates the inability of correcting measurement errors to the absence of long-range entanglement through  $\sigma_{e_0}$  spins.

- 
- [1] G.-Y. Zhu, N. Tantivasadakarn, A. Vishwanath, S. Trebst, and R. Verresen, Nishimori’s cat: stable long-range entanglement from finite-depth unitaries and weak measurements (2022), [arXiv:2208.11136 \[quant-ph\]](#).
  - [2] J. Y. Lee, W. Ji, Z. Bi, and M. P. A. Fisher, Decoding measurement-prepared quantum phases and transitions: from ising model to gauge theory, and beyond (2022), [arXiv:2208.11699 \[cond-mat.str-el\]](#).
  - [3] J. B. Kogut, An introduction to lattice gauge theory and spin systems, *Rev. Mod. Phys.* **51**, 659 (1979).
  - [4] S. Elitzur, Impossibility of spontaneously breaking local symmetries, *Phys. Rev. D* **12**, 3978 (1975).
  - [5] E. Dennis, A. Kitaev, A. Landahl, and J. Preskill, Topological quantum memory, *Journal of Mathematical Physics* **43**, 4452 (2002).
  - [6] H. Nishimori, Internal Energy, Specific Heat and Correlation Function of the Bond-Random Ising Model, *Progress of Theoretical Physics* **66**, 1169 (1981).
  - [7] C. Wang, J. Harrington, and J. Preskill, Confinement-higgs transition in a disordered gauge theory and the accuracy threshold for quantum memory, *Annals of Physics* **303**, 31 (2003).
